# Supplementary material for: Safe and Efficient Switching Controller Design for Partially Observed Linear-Gaussian Systems
Source: arXiv:2212.04140 source file (2023-03-27)
Supplement: Supplementary file 1 [file ifacconf_noappendix.tex]

\input{ifacconf.tex}
